# Supplementary material for: The "Giant Virus Finder" Discovers an Abundance of Giant Viruses in the Antarctic Dry Valleys
Source: arXiv:1503.05575 ancillary file (2015-11-24)
Supplement: Supplementary file 1 [file Supporting.pdf]

**Supplementary information for the article: "The Giant Virus Finder Discovers an Abundance of Giant Viruses in the Antarctic Dry Walleys" by Csaba Kerepesi & Vince Grolmusz**

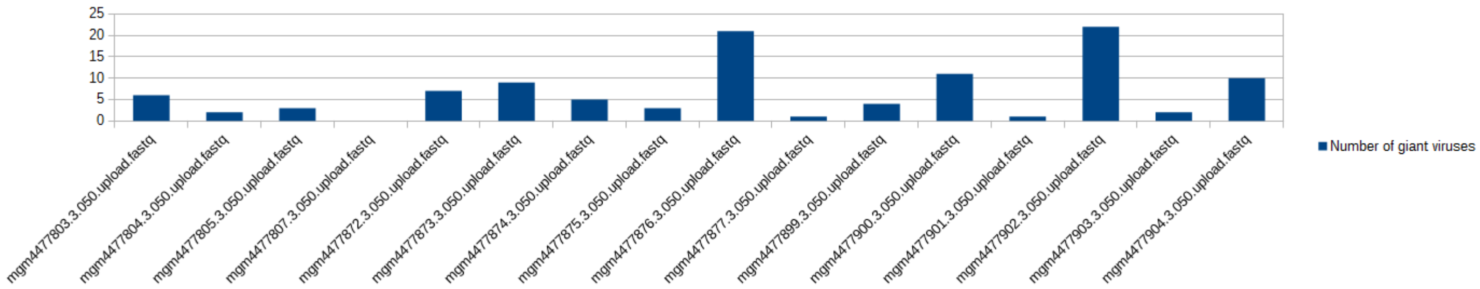


Figure S1: The number of giant virus reads found is visualized in each metagenome deposited at http://metagenomics.anl.gov/metagenomics.cgi?page=MetagenomeProject&project=2997. This figure is the metagenome-filename labelled version of Figure 1 in the main text.

**TABLE S1: GIANT VIRUS FINDER WORKFLOW ON THE COMMAND LEVEL:**

```
- Prerequisites: Perl 5.14.2 or later, Python 2.7, Biopython 1.5 or later
- Start from the ~/GiantVirusFinder directory
- Download all Giant Virus Finder files to GiantVirusFinder directory

***Making Giant Virus Toplist:
- mkdir AllVirusGenome
- wget ftp://ftp.ncbi.nlm.nih.gov/genomes/Viruses/all.fna.tar.gz
- tar xvzf
- cd ..
- mkdir TopGiants-gb-300k
- cd TopGiants-gb-300k
- python ../TopGiantsEntrez.py 1
- cd ..
- perl TopGiants.pl TopGiants-gb-300k/TopGiants-gb-300k.csv 300000

***Installing Stand alone UNIX BLAST:
- cd ~
- wget ftp://ftp.ncbi.nlm.nih.gov/blast/executables/LATEST/ncbi-blast-2.2.30+-x64-
linux.tar.gz
- tar xvzf
- mkdir ncbi-blast-2.2.30+/db
- cd ncbi-blast-2.2.30+/db
- wget ftp://ftp.ncbi.nlm.nih.gov/blast/db/nt*
- ls *.gz | while read line; do tar xvzf $line; done
- cd  ~/GiantVirusFinder

***Building metagenome database:
- mkdir 16SoilMetagenome
- cd 16SoilMetagenome
- Download the 16 soil metagenomes:
http://metagenomics.anl.gov/metagenomics.cgi?page=MetagenomeProject&project=2997
- Convert the fastq files to fasta
- ls *.fasta > ../mgm.list
- ls *.fasta | while read line; do ~/ncbi-blast-2.2.30+/bin/makeblastdb -dbtype nucl -
in $line -out ~/ncbi-blast-2.2.30+/db/$line; done
- cd ..

***Giant Virus Finding, Phase1:
- mkdir Giants-in-16Soil-metagenomes
- perl Phase1Blast-MultiCore.pl Giants-in-16Soil-metagenomes > Giants-in-16Soil-
metagenomes/log-Phase1Blast-MultiCore.pl.txt
- perl Concat.pl Giants-in-16Soil-metagenomes
- perl GetCandidateReads.pl Giants-in-16Soil-metagenomes 16SoilMetagenome

***Giant Virus Finding, Phase2:
- perl Phase2Blast-MultiCore.pl Giants-in-16Soil-metagenomes > Giants-in-16Soil-
metagenomes/log-Phase2Blast-MultiCore.pl.txt
- perl GiantVirusFinder-Multi.pl Giants-in-16Soil-metagenomes 0.2
- perl CountGiants.pl Giants-in-16Soil-metagenomes 0.2
- perl blastx-Multi.pl Giants-in-16Soil-metagenomes 0.2
```

Table S3: The list of viruses with larger than 300 kbp genomes

| | Sequence title | Length | Segm. | Accession |
|---|---|---|---|---|
| 1 | Pandoravirus salinus, complete genome | 2473870 | 1 | NC_022098.1 |
| 2 | Pandoravirus inopinatum isolate KlaHel, complete genome | 2243109 | 1 | NC_026440.1 |
| 3 | Pandoravirus dulcis, complete genome | 1908524 | 1 | NC_021858.1 |
| 4 | Megavirus chiliensis, complete genome | 1259197 | 1 | NC_016072.1 |
| 5 | Megavirus courdo11, complete genome | 1246126 | 1 | JX975216.1 |
| 6 | Megavirus terra1 genome | 1244621 | 1 | NC_023640.1 |
| 7 | Megavirus lba isolate LBA111, complete genome | 1230522 | 1 | NC_020232.1 |
| 8 | Samba virus, partial genome | 1212735 | 1 | KF959826.1 |
| 9 | Acanthamoeba castellanii mamavirus strain Hal-V, complete genome | 1191693 | 1 | JF801956.1 |
| 10 | Acanthamoeba polyphaga mimivirus, complete genome | 1181549 | 1 | NC_014649.1 |
| 11 | Hirudovirus strain Sangsue, complete genome | 1181042 | 1 | KF493731.1 |
| 12 | Mimivirus terra2 genome | 1168989 | 1 | NC_023639.1 |
| 13 | Acanthamoeba polyphaga moumouvirus, complete genome | 1021348 | 1 | NC_020104.1 |
| 14 | UNVERIFIED: Moumouvirus goulette, complete genome | 1016844 | 1 | KC008572.1 |
| 15 | Acanthamoeba polyphaga mimivirus isolate M4, complete genome | 981813 | 1 | JN036606.1 |
| 16 | Acanthamoeba polyphaga lentillevirus contig00005, whole genome shotgun sequence | 788571 | 1 | AFYC01000005.1 |
| 17 | Cafeteria roenbergensis virus BV-PW1, complete genome | 617453 | 1 | NC_014637.1 |
| 18 | Pithovirus sibericum isolate P1084-T, complete genome | 610033 | 1 | NC_023423.1 |
| 19 | Cotesia congregata virus complete genome, segment Circle21 | 567670 | 30 | NC_006652.1 |
| 20 | Megavirus courdo7 isolate Mv13-c7, partial genome | 529672 | 1 | JN885991.1 |
| 21 | Cotesia congregata bracovirus proviral locus 2 (PL2) | 522749 | 1 | HF586473.1 |
| 22 | Bacillus phage G, complete genome | 497513 | 1 | NC_023719.1 |
| 23 | Phaeocystis globosa virus 12T, *** SEQUENCING IN PROGRESS ***, 3 unordered pieces | 460002 | 1 | HQ634147.1 |
| 24 | Phaeocystis globosa virus strain 16T, complete genome | 459984 | 1 | NC_021312.1 |
| 25 | Phaeocystis globosa virus 14T, *** SEQUENCING IN PROGRESS ***, 3 unordered pieces | 452892 | 1 | HQ634144.1 |
| 26 | Emiliania huxleyi virus 207, *** SEQUENCING IN PROGRESS ***, 16 unordered pieces | 421891 | 1 | JF974317.1 |

| | | | | |
|---|---|---|---|---|
| 27 | Emiliania huxleyi virus 208, *** SEQUENCING IN PROGRESS ***, 17 unordered pieces | 411003 | 1 | JF974318.1 |
| 28 | Emiliania huxleyi virus 202, *** SEQUENCING IN PROGRESS ***, 12 unordered pieces | 407516 | 1 | HQ634145.1 |
| 29 | Emiliania huxleyi virus 86 isolate EhV86 | 407339 | 1 | AJ890364.1 |
| 30 | Emiliania huxleyi virus 86, complete genome | 407339 | 1 | NC_007346.1 |
| 31 | Emiliania huxleyi virus 201, *** SEQUENCING IN PROGRESS ***, 7 unordered pieces | 407301 | 1 | JF974311.1 |
| 32 | Emiliania huxleyi virus 164 partial genome sequence | 401558 | 1 | KF481688.1 |
| 33 | Emiliania huxleyi virus 18 partial genome sequence | 400762 | 1 | KF481685.1 |
| 34 | Emiliania huxleyi virus 203, *** SEQUENCING IN PROGRESS ***, 7 unordered pieces | 400520 | 1 | JF974291.1 |
| 35 | Emiliania huxleyi virus 156 partial genome sequence | 400341 | 1 | KF481687.1 |
| 36 | Emiliania huxleyi virus 145 partial genome sequence | 399873 | 1 | KF481686.1 |
| 37 | Emiliania huxleyi virus 88, *** SEQUENCING IN PROGRESS ***, 8 unordered pieces | 397298 | 1 | JF974310.1 |
| 38 | Emiliania huxleyi virus 84, *** SEQUENCING IN PROGRESS ***, 9 unordered pieces | 396620 | 1 | JF974290.1 |
| 39 | Insectomime virus strain V478, partial genome | 386631 | 1 | KF527888.1 |
| 40 | Insectomime virus V478 genomic scaffold, scaffold00001, whole genome shotgun sequence | 382785 | 1 | HG428764.1 |
| 41 | Tunisvirus fontaine2 strain U484, complete genome | 380011 | 1 | KF483846.1 |
| 42 | Emiliania huxleyi virus 99B1 draft genome sequence | 376759 | 1 | FN429076.1 |
| 43 | Cannes 8 virus, complete genome | 374041 | 1 | KF261120.1 |
| 44 | Aureococcus anophagefferens virus isolate BtV-01, complete genome | 370920 | 1 | NC_024697.1 |
| 45 | Melbournevirus isolate 1, complete genome | 369360 | 1 | NC_025412.1 |
| 46 | Paramecium bursaria Chlorella virus NY2A Chlorella virus NY2A ctg_13 genomic sequence | 368683 | 1 | DQ491002.1 |
| 47 | Paramecium bursaria Chlorella virus NY2A, complete genome | 368683 | 1 | NC_009898.1 |
| 48 | Marseillevirus marseillevirus strain T19, complete genome | 368454 | 1 | NC_013756.1 |
| 49 | Canarypox virus strain ATCC VR-111, complete genome | 359853 | 1 | AY318871.1 |
| 50 | Canarypox virus, complete genome | 359853 | 1 | NC_005309.1 |
| 51 | Cronobacter phage vB_CsaM_GAP32, complete genome | 358663 | 1 | NC_019401.1 |
| 52 | Escherichia phage 121Q, complete genome | 348532 | 1 | NC_025447.1 |
| 53 | Paramecium bursaria Chlorella virus NYs1, partial genome | 348463 | 1 | JX997183.1 |

| | | | | |
|---|---|---|---|---|
| 54 | Escherichia phage PBECO 4, complete genome | 348113 | 1 | KC295538.1 |
| 55 | Lausannevirus, complete genome | 346754 | 1 | NC_015326.1 |
| 56 | Lausannevirus isolate 7715, complete genome | 346754 | 1 | HQ113105.1 |
| 57 | Klebsiella phage K64-1 DNA, complete genome | 346602 | 1 | AB897757.1 |
| 58 | Enterobacteria phage vB_KleM-RaK2, complete genome | 345809 | 1 | NC_019526.1 |
| 59 | Moumouvirus Monve isolate Mv13-mv, partial genome | 345413 | 1 | JN885998.1 |
| 60 | Paramecium bursaria Chlorella virus IL-5-2s1, partial genome | 345255 | 1 | JX997170.1 |
| 61 | Paramecium bursaria Chlorella virus NY-2B, partial genome | 344863 | 1 | JX997182.1 |
| 62 | Organic Lake phycodnavirus 1 genomic sequence | 344723 | 1 | HQ704802.1 |
| 63 | Paramecium bursaria Chlorella virus AR158, complete genome | 344691 | 1 | NC_009899.1 |
| 64 | Paramecium bursaria Chlorella virus AR158 genomic sequence | 344691 | 1 | DQ491003.2 |
| 65 | Paramecium bursaria Chlorella virus MA-1D, partial genome | 339653 | 1 | JX997172.1 |
| 66 | Paramecium bursaria Chlorella virus MA-1E, partial genome | 339391 | 1 | JX997173.1 |
| 67 | Ectocarpus siliculosus virus, complete genome | 335593 | 1 | AF204951.2 |
| 68 | Ectocarpus siliculosus virus 1, complete genome | 335593 | 1 | NC_002687.1 |
| 69 | Enterobacteria phage RB3, complete genome | 333581 | 2 | NC_025419.1 |
| 70 | Paramecium bursaria Chlorella virus AN69C, partial genome | 332309 | 1 | JX997153.1 |
| 71 | Paramecium bursaria Chlorella virus 1 (PBCV-1), complete genome | 330611 | 1 | JF411744.1 |
| 72 | Paramecium bursaria Chlorella virus 1, complete genome | 330611 | 1 | NC_000852.5 |
| 73 | Paramecium bursaria Chlorella virus CVR-1, partial genome | 330002 | 1 | JX997164.1 |
| 74 | Paramecium bursaria Chlorella virus Can18-4, partial genome | 329890 | 1 | JX997157.1 |
| 75 | Paramecium bursaria Chlorella virus NE-JV-4, partial genome | 328315 | 1 | JX997179.1 |
| 76 | Acanthocystis turfacea Chlorella virus MN0810.1, partial genome | 327406 | 1 | JX997174.1 |
| 77 | Paramecium bursaria Chlorella virus AP110A, partial genome | 327349 | 1 | JX997154.1 |
| 78 | Paramecium bursaria Chlorella virus CVM-1, partial genome | 327107 | 1 | JX997163.1 |

| | | | | |
|---|---|---|---|---|
| 79 | Paramecium bursaria Chlorella virus CVA-1, partial genome | 326592 | 1 | JX997159.1 |
| 80 | Paramecium bursaria Chlorella virus NE-JV-1, partial genome | 326559 | 1 | JX997176.1 |
| 81 | Paramecium bursaria Chlorella virus NW665.2, partial genome | 325996 | 1 | JX997181.1 |
| 82 | Acanthocystis turfacea Chlorella virus NTS-1, partial genome | 323517 | 1 | JX997180.1 |
| 83 | Paramecium bursaria Chlorella virus IL-3A, partial genome | 323497 | 1 | JX997169.1 |
| 84 | Paramecium bursaria Chlorella virus FR483, complete genome | 321240 | 1 | NC_008603.1 |
| 85 | Acanthocystis turfacea Chlorella virus TN603.4.2, partial genome | 320880 | 1 | JX997186.1 |
| 86 | Acanthocystis turfacea Chlorella virus NE-JV-2, partial genome | 319583 | 1 | JX997177.1 |
| 87 | Paramecium bursaria Chlorella virus CVB-1, partial genome | 319457 | 1 | JX997160.1 |
| 88 | Paramecium bursaria Chlorella virus CVG-1, partial genome | 318742 | 1 | JX997161.1 |
| 89 | Pseudomonas phage 201phi2-1, complete genome | 316674 | 1 | NC_010821.1 |
| 90 | Acanthocystis turfacea Chlorella virus GM0701.1, partial genome | 315239 | 1 | JX997168.1 |
| 91 | Paramecium bursaria chlorella virus MT325 genomic sequence | 314335 | 1 | DQ491001.1 |
| 92 | Paramecium bursaria Chlorella virus OR0704.2.2, partial genome | 313584 | 1 | JX997184.1 |
| 93 | Acanthocystis turfacea Chlorella virus OR0704.3, partial genome | 311647 | 1 | JX997185.1 |
| 94 | Paramecium bursaria Chlorella virus CvsA1, partial genome | 311223 | 1 | JX997165.1 |
| 95 | Pseudomonas phage PhiPA3, complete genome | 309208 | 1 | HQ630627.1 |
| 96 | Paramecium bursaria Chlorella virus CviKI, partial genome | 309195 | 1 | JX997162.1 |
| 97 | Choristoneura biennis entomopoxvirus ‘L’, complete genome | 307691 | 1 | NC_021248.1 |
| 98 | Penguinpox virus isolate PSan92, complete genome | 306862 | 1 | NC_024446.1 |
| 99 | Acanthocystis turfacea Chlorella virus Can0610SP, partial genome | 306752 | 1 | JX997156.1 |
| 100 | Paramecium bursaria Chlorella virus CZ-2, partial genome | 305715 | 1 | JX997166.1 |
| 101 | White spot syndrome virus, complete genome | 305119 | 1 | AF332093.3 |

| | | | | |
|---|---|---|---|---|
| 102 | Shrimp white spot syndrome virus, complete genome | 305108 | 1 | NC_003225.2 |
| 103 | Sequence 1 from Patent WO0138351 | 305107 | 1 | AX151396.1 |
| 104 | Paramecium bursaria Chlorella virus Fr5L, partial genome | 303810 | 1 | JX997167.1 |
| 105 | Emiliania huxleyi virus PS401, *** SEQUENCING IN PROGRESS ***, 13 unordered pieces | 301520 | 1 | HQ634146.1 |

Table S4: The giant viruses found by the "Giant Virus Finder". DNA sequences found *k* times in the samples are denoted by '*k* x "name of species"'.

| Source description * | Source location and taxa found* |
|---|---|
| | |
| **Deserts and xeric shrubland** | **Lake Bonney Valley, Antarctica** |
| mgm4477803.3.050 | Organic Lake phycodnavirus |
| | Aureococcus anophagefferens virus |
| | Megavirus terra1 |
| | Klebsiella phage K64-1 |
| | Acanthamoeba polyphaga moumouvirus |
| | Acanthocystis turfacea Chlorella virus |
| | |
| **Temperate grasslands** | **Konza Prairie LTER, Kansas, USA** |
| mgm4477804.3.050 | Samba virus |
| | Pandoravirus salinus |
| | |
| **Deserts and xeric shrubland** | **Mojave Desert, California, USA** |
| mgm4477805.3.050 | 2 x Pandoravirus inopinatum |
| | Pandoravirus salinus |
| | |
| **Trop. & subtrop. broadleaf forest** | **Manu National Park, Peru** |
| mgm4477807.3.050 | |
| | |
| **Deserts and xeric shrubland** | **Chihuahuan Desert, Galisteo, NM, USA** |
| mgm4477872.3.050 | 2 x Acanthamoeba polyphaga moumouvirus |
| | Ectocarpus siliculosus virus |
| | Moumouvirus Monve |
| | Pandoravirus dulcis |
| | Samba virus |
| | Megavirus Iba |
| | |
| **Deserts and xeric shrubland** | **Chihuahuan Desert, Sevilleta, NM, USA** |
| mgm4477873.3.050 | 3 x Megavirus terra1 |
| | Megavirus Iba |
| | Paramecium bursaria Chlorella virus |
| | Samba virus |
| | Mimivirus terra2 |

| | |
|---|---|
| | Megavirus Iba |
| | Megavirus courdo11 |
| | |
| **Tundra** | **Toolik Lake LTER, Alaska, USA** |
| mgm4477874.3.050 | 2 x Acanthamoeba polyphaga moumouvirus |
| | 2 x Cafeteria roenbergensis virus |
| | Megavirus terra1 |
| | |
| **Trop. & subtrop. broadleaf forest** | **Misiones, Argentina** |
| mgm4477875.3.050 | Pandoravirus inopinatum |
| | Acanthamoeba polyphaga moumouvirus |
| | Pandoravirus dulcis |
| | |
| **Temperate coniferous forest** | **Bonanza Creek LTER, Alaska, USA** |
| mgm4477876.3.050 | 8 x Megavirus terra1 |
| | Paramecium bursaria Chlorella virus |
| | 3 x Samba virus |
| | Megavirus Iba |
| | Pandoravirus dulcis |
| | Acanthocystis turfacea Chlorella virus |
| | Acanthamoeba polyphaga moumouvirus |
| | Klebsiella phage K64-1 |
| | Cronobacter phage vB_CsaM_GAP32 |
| | 2 x Moumouvirus Monve |
| | Cafeteria roenbergensis virus |
| | |
| **Temperate coniferous forest** | **Calhoun Experimental Forest, SC, USA** |
| mgm4477877.3.050 | Cafeteria roenbergensis virus |
| | |
| **Temperate coniferous forest** | **Duke Forest, North Carolina, USA** |
| mgm4477899.3.050 | Samba virus |
| | Cafeteria roenbergensis virus |
| | Pandoravirus salinus |
| | Pandoravirus dulcis |
| | |
| **Deserts and xeric shrubland** | **Garwood Valley, Antarctica** |
| mgm4477900.3.050 | Mimivirus terra2 |

| | |
|---|---|
| | Samba virus |
| | Acanthamoeba polyphaga moumouvirus |
| | 2 x Cafeteria roenbergensis virus |
| | 5 x Megavirus terra1 |
| | Megavirus chiliensis |
| | |
| **Deserts and xeric shrubland** | **Lake Bonney Valley, Antarctica** |
| mgm4477901.3.050 | Cronobacter phage PBECO 4 |
| | |
| **Deserts and xeric shrubland** | **Lake Fryxell Valley, Antarctica** |
| mgm4477902.3.050 | 3 x Acanthamoeba polyphaga moumouvirus |
| | 4 x Megavirus terra1 |
| | 4 x Pandoravirus inopinatum |
| | Paramecium bursaria Chlorella virus |
| | 2 x Cafeteria roenbergensis virus |
| | 2 x Moumouvirus Monve |
| | 2x Samba virus |
| | 2 x Pandoravirus dulcis |
| | 2 x Megavirus Iba |
| | |
| **Deserts and xeric shrubland** | **Lake Hoare Valley, Antarctica** |
| mgm4477903.3.050 | Pandoravirus dulcis |
| | Pandoravirus salinus |
| | |
| **Deserts and xeric shrubland** | **Wright Valley, Antarctica** |
| mgm4477904.3.050 | Mimivirus terra2 |
| | Megavirus terra1 |
| | Pandoravirus inopinatum |
| | Pandoravirus salinus |
| | Hirudovirus strain Sangsue |
| | 2 x Pandoravirus dulcis |
| | Moumouvirus Monve |
| | Paramecium bursaria Chlorella virus |
| | Acanthamoeba polyphaga moumouvirus |
